# Supplementary material for: Approximate Hofstadter- and Kapit-Mueller-like parent Hamiltonians for Laughlin states on fractals
Source: arXiv:2301.09971 ancillary file (2023-06-29)
Supplement: Supplementary file 1 [file readme.pdf]

# Supplementary material to “Approximate Hofstadter- and Kapit-Mueller-like parent Hamiltonians for Laughlin states on fractals”

Błażej Jaworowski, Michael Iversen, and Anne E. B Nielsen

*Department of Physics and Astronomy, Aarhus University, DK-8000 Aarhus C, Denmark*

As Supplementary Material to our paper, we provide further details on our results. Here, we explain the contents of the data files.

## I. THE MODEL WAVEFUNCTIONS

The two subdirectories `[lattice]` (i.e. `triangle` and `carpet`) of the main directory contain files named `positions.txt`. These files contain the site positions for the triangle and the carpet, respectively. The first and second column of each file contains  $x$  and  $y$  coordinates, respectively, while each row corresponds to a different site.

Both `[lattice]` subdirectories have further subdirectories `[lattice]/M0=[number]` (e.g. `triangle/M0=4`) corresponding to different initial particle numbers  $M_0$ . Each of these contains a subdirectory `[lattice]/M0=[number]/wfn`. In each of these subdirectories, there is a file `density.txt`, containing the particle density profile of the state without anyons at  $M = M_0$ . The number in each line is the particle density at a given site, according to the ordering of sites in a corresponding `positions.txt` file. In most of the `[lattice]/M0=[number]/wfn` directories, there are also additional files:

1. `anyondensity.txt` – describing the particle density at  $M = M_0 - 1$  and two anyons placed as in Fig. 6 of the main text,
2. `excessdensity.pdf` – a plot of excess particle density (a difference between the numbers from `anyondensity.txt` and `density.txt`).

In addition, the main directory has a subdirectory `wfn_example`, where one can find an example Python script `laughlin_anyons.py` generating the model wavefunction with two anyons and the corresponding particle density. As an input, the code takes the positions file `positions.txt` and the basis file `basis.txt`. In the latter, each row lists the occupied sites in a given configuration. The output is the file `wfn.txt` (where the first and second column lists the real and imaginary coefficients of the wavefunction, respectively, according to the ordering of configurations in `basis.txt`), as well as the density file `anyondensity.txt`. The `basis.txt` file is generated by the exact diagonalization code (not included here). The example input and output is provided for an  $M_0 = 3$ ,  $M = 2$  system on a triangle. For comparison, we also provide a file `gs.txt`, which is a ground state of the  $r = 1.1$   $M_0 = 3$  Hamiltonian with  $M = 2$  particles

and two  $V = 1000$  potentials (whose positions coincide with anyons in the model wavefunction), written in the same basis. The squared overlap between these states, which can be computed using the `overlap.py` script, is  $|\langle \psi | \tilde{\Psi} \rangle|^2 \approx 0.979$ .

## II. THE HAMILTONIANS

In each `[lattice]/M0=[number]` subdirectory, in addition to the results for model wavefunctions, there are also further subdirectories `[lattice]/M0=[number]/[type]`, corresponding to the Hamiltonians generated for different types of clusters  $S_\alpha$  (e.g. `triangle/M0=4/r=1.1`). They contain the coefficients of the Hamiltonians and some further results for each case. For each case, we provide the data for one Hamiltonian. In most of the cases, the chosen Hamiltonian is the one with  $d$  value yielding maximum overlap. The only exceptions are the NN-clique cases on the carpet, where  $d$  is not used, and the Hamiltonian is defined by taking only the eigenvector of each  $\mathbf{B}^{(\alpha)}$  corresponding to the lowest eigenvalue.

In each of the `[lattice]/M0=[number]/[type]` subdirectories, there are several files:

1. `hoppings.txt` – a file describing the hopping terms of the Hamiltonian. The header contains information about  $d$  used. If the Hamiltonian is written as

$$H = \sum_{j < k} [\tilde{t}_{jk} a_j^\dagger a_k + \text{H.c.}] + \sum_j \epsilon_j n_j, \quad (1)$$

with  $\tilde{t}_{jk}$  being a complex number, then the columns of the file contain (starting from the left):  $j$ ,  $k$ ,  $\text{Re}\tilde{t}_{jk}$ ,  $\text{Im}\tilde{t}_{jk}$ . The  $j$ th ( $k$ th) site is the site whose coordinates are given in the  $j$ th ( $k$ th) row of `positions.txt` file for a given lattice type. Note that (1) is equivalent to Eq. (4) in the main text, but the notation is a bit different.

2. `onsite.txt` – contains the onsite potentials  $\epsilon_j$  (each row contains the numbers  $j$  and  $\epsilon_j$ ), with sites ordered in the same way as in the corresponding `positions.txt` file.
3. `hamiltonian.pdf` – a plot of the Hamiltonian terms in a similar way as in Fig. 3 of the main text. The arrows denote the hoppings  $\tilde{t}_{jk} = t_{jk} e^{i\phi_{jk}}$ , with strength  $t_{jk}$  given by intensity and phase  $\phi_{jk}$

by color. The dots symbolize the onsite potentials  $\epsilon_j$ , with sizes representing their strength. The terms are rescaled so that the highest  $t_{jk}$  is unity. The numbers on the plot are the site indices according to `positions.txt`.

4. `spectrum.txt` – the energy spectrum of the Hamiltonian at  $M = M_0$  particles (lowest 20 eigenvalues).
5. `density.txt` – the particle density in the ground state at  $M = M_0$  particles.
6. `overlaps.txt` – squared overlaps of the four lowest energy eigenstates at  $M = M_0$  particles with the corresponding model state without anyons, i.e. (2) in the main text.
7. `1partspectrum.txt` – the energy spectrum of the Hamiltonian at  $M = 1$  particle.
8. `1partspectrum.pdf` – plot of the energy spectrum of the Hamiltonian at  $M = 1$  particle.

Most of the `[lattice]/M0=[number]/[type]` directories contain also the results for  $M = M_0 - 1$  particles and two  $V = 1000$  potentials placed as in Fig. 6 of the main text:

1. `anyonspectrum.txt` – the energy spectrum of the Hamiltonian (lowest 20 eigenvalues).
2. `anyondensity.txt` – the particle density in the ground state.
3. `anyonoverlaps.txt` – the squared overlaps between the four lowest energy eigenstates and the model wavefunction given by (3) in the main text.
4. `excessdensity.txt` – the plot of the excess density of the ground state relative to the  $M = M_0$  ground state.

Note that only the plot `hamiltonian.pdf` contains rescaled coefficients (to make the different plots consistent with each other) – the values in `hoppings.txt` and `onsite.txt` are not rescaled. All the energy spectra are also obtained without rescaling.

### III. BRAIDING

In addition to `triangle` and `carpet` folders, the main directory contains also the `braiding` subdirectory, which contains the results of the braiding calculations for the triangle with  $M_0 = 6$ . Each of its subfolders `braiding/path[npath]_[type]` (e.g. `braiding/path1_r=1.1`) contains the results for a different case. Here, `[npath]` equal to 1 or 2 corresponds to the paths from Figs. 8 and 10 of the main text, respectively, while `[type]` “wfn” means the model wavefunction and “r=...” denotes the Hamiltonian created at given  $r$ .

The directories corresponding to model wavefunctions (`braiding/path[npath]_wfn`) contain the following files:

1. `phases.txt` – the total braiding phase as a function of the number of interpolation steps. The first column is  $n_{\text{interp}}$  and the second is  $\gamma_{\text{br}}/\pi$ .
2. `animation_ex_wfn_path[npath].mp4`, `animation_ab_wfn_path[npath].mp4` – the animations of the excess density throughout the exchange and AB paths, respectively, at  $n_{\text{interp}} = 100$ . The red crosses denote  $w_1$  and  $w_2$ .

The directories corresponding to Hamiltonians:

`braiding/path[npath]_r=1.1` and

`braiding/path[npath]_r=4.1`,

contain further subdirectories:

`braiding/path[npath]_[type]/V=[potential]`, which store the results at a given potential strength  $V$  (e.g. `braiding/path1_r=1.1/V=10`). Inside each of them, there are the following files:

1. `phases.txt` – the total braiding phase as a function of the number of interpolation steps. The first column is  $n_{\text{interp}}$  and the second is  $\gamma_{\text{br}}/\pi$ .
2. `animation_ex...`, `animation_ab...` – the animation of the excess density throughout the exchange and AB phase calculation, respectively, at maximum considered  $n_{\text{interp}}$ . The red crosses denote the positions of potentials.
3. `spectrum_ex.txt`, `spectrum_ab.txt` – the energy spectra (lowest 10 eigenvalues) at each step of the exchange and AB paths, respectively. The first number in each row is  $t$ , the other are the energy eigenvalues.
4. `spectrum_ex.txt`, `spectrum_ab.txt` – the plots of the energy spectra at each step of the exchange and AB paths, respectively.
